# Supplementary material for: Deformation Driven Suction Cups: A Mechanics-Based Approach to Wearable Electronics
Source: arXiv:2508.11838 source file (2025-09-08)
Supplement: Supplementary file 1 [file sucky.pdf]

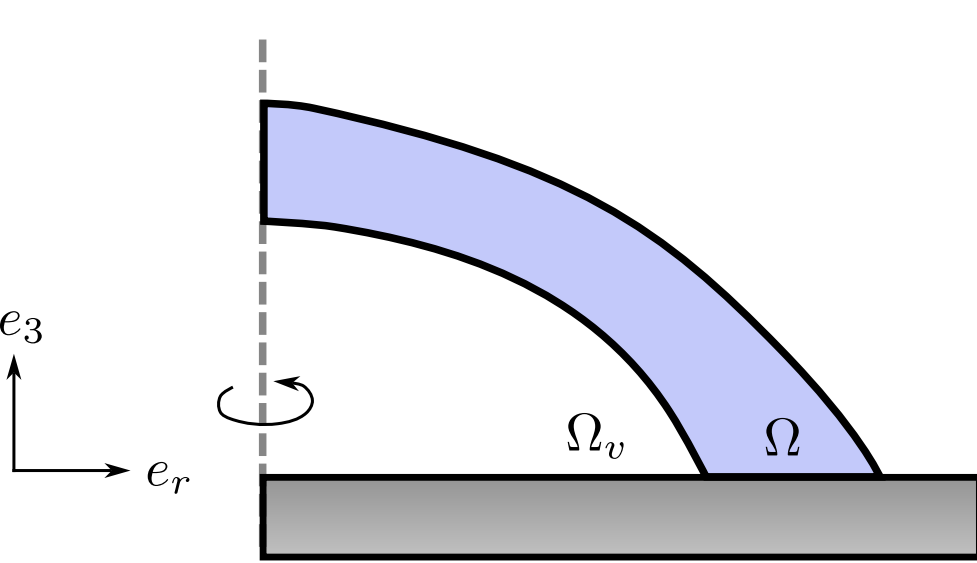

Reference

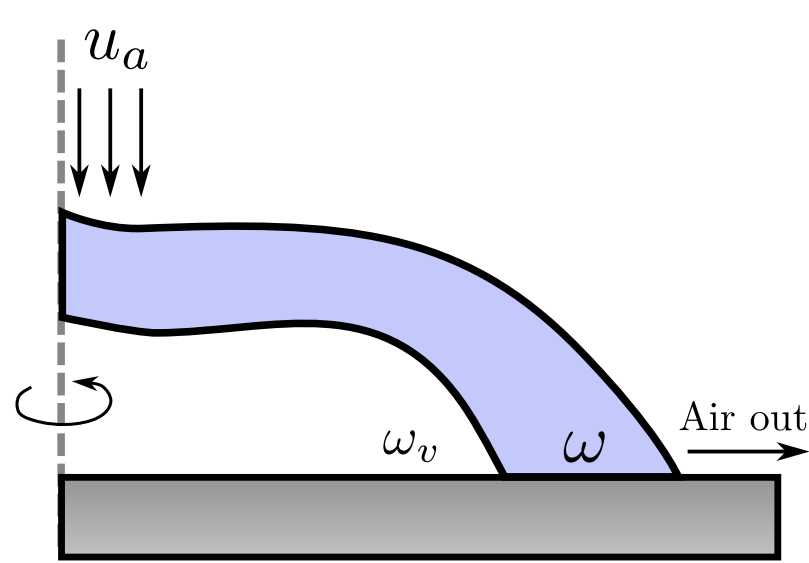

Loaded

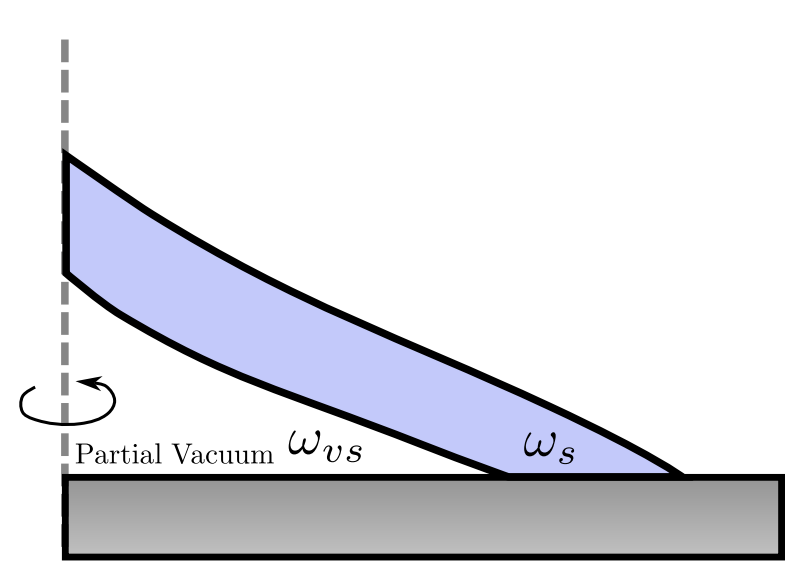

Unloaded, Suction
