# Supplementary material for: Deformation Driven Suction Cups: A Mechanics-Based Approach to Wearable Electronics
Source: arXiv:2508.11838 source file (2025-09-08)

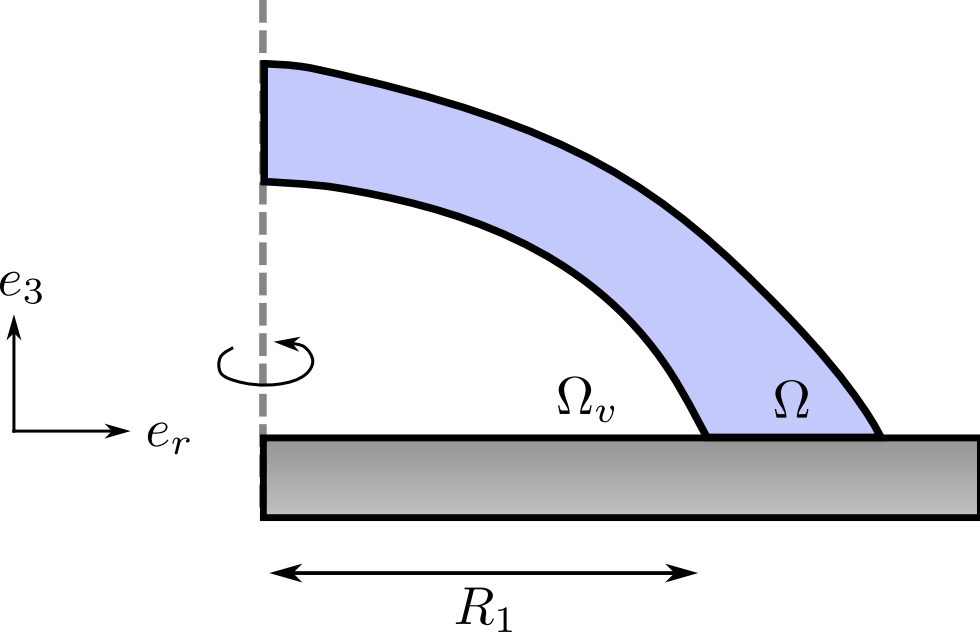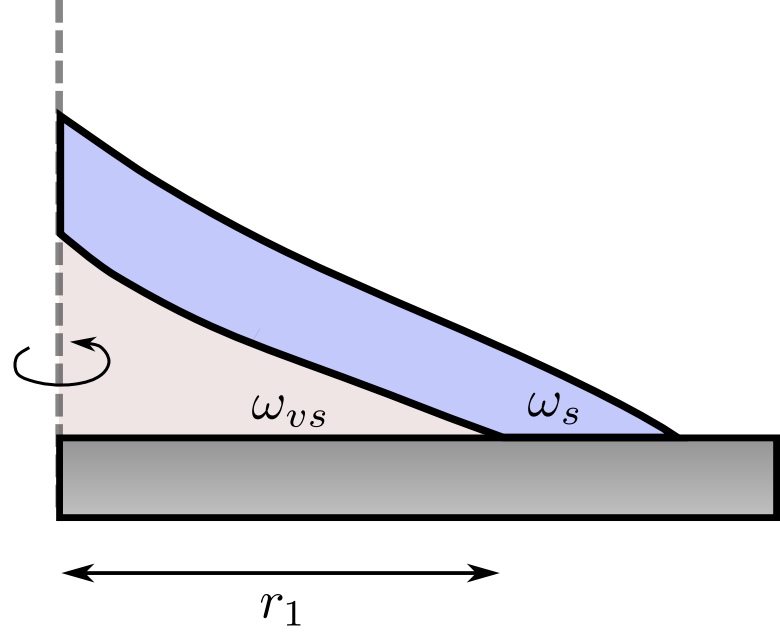

Supplement: Supplementary file 2 [file suction_dia.pdf]
